# Supplementary material for: Theoretical Insights into Inorganic Antiperovskite Nitrides (X$_3$NA; X = Mg, Sr, Ca, Ba; A = Sb, As): An Emerging Class of Materials for Photovoltaics
Source: arXiv:2404.16494 source file (2024-04-25)
Supplement: Supplementary file 1 [file SI.pdf]

# Supplemental Material for "Theoretical Insights into Inorganic Antiperovskite Nitrides ($X_3NA$; X = Mg, Sr, Ca, Ba; A = Sb, As): An Emerging Class of Materials for Photovoltaics"

Sanchi Monga*,[1] Manjari Jain,[1] Sajjan Sheoran,[1]
Claudia Draxl*,[2] and Saswata Bhattacharya[1]

[1]*Department of Physics, Indian Institute of Technology Delhi, New Delhi 110016, India*
[2]*Institut für Physik and IRIS Adlershof,*
*Humboldt-Universität zu Berlin, 12489 Berlin, Germany*

## I. COMPUTATIONAL DETAILS

The Density Functional Theory (DFT) [1, 2] calculations were performed using the Vienna *Ab initio* Simulation Package (VASP) [3, 4], which implements the Projector Augmented Wave (PAW)[3, 5] pseudopotential method, and the full-potential all-electron code **exciting**[6], which implements linearized augmented planewave methods. Starting from the experimentally determined structures [7–9] (see Table S1), the respective atomic positions were optimized with VASP using the generalized gradient approximation within the Perdew-Burke-Ernzerhof (PBE) parametrization [10] until the Hellmann-Feynman forces were less than 0.01 eV/Å. A convergence threshold of 0.01 meV was used for the total energy, and a kinetic energy cutoff of 550 eV. Γ-centered 6×6×6, 4×4×3, and 4×4×4 $k$-grids were employed for the Brillouin zone integration in the $Pm\overline{3}m$, $Pbnm$ and $P6_3/mmc$ phases, respectively. The dynamical stability of these materials was checked by computing the phonon dispersions with $2 \times 2 \times 2$ supercells using the PHONOPY [11, 12] package. In **exciting**, muffin-tin radii of 1.89, 2.01, 2.07, and 2.47 Bohr were used for N, Mg, Sr, and Sb, respectively, and a basis set cutoff of $\mathrm{R_{MT}|G + k|_{max}} = 8.0$. Band-gap calculations have been carried out with different exchange-correlation functionals. As expected, PBE underestimates them, but HSE06 [13] reproduces the experimental values, as shown by both VASP and **exciting**. HSE06 is then used to calculate the electronic band structures and densities of states. Spin-orbit coupling (SOC) has been included in all calculations. The effective carrier masses were estimated by parabolic fitting of the band edges using SUMO [14]. Single-shot $G_0W_0$ [15, 16] with HSE06 as a starting point was used to account for many-body effects. The number of empty states used in the $G_0W_0$ calculations were carefully converged (see Section V). Electron-hole interactions were incorporated by solving the Bethe–Salpeter equation (BSE) [17–19] within the Tamm-Dancoff approximation (TDA). 22 occupied and unoccupied orbitals have been used to construct the BSE Hamiltonian. The ionic contribution to the dielectric screening was estimated using density functional perturbation theory (DFPT) [20] with 20×20×20, 16×16×16, and 14×14×10 $k$-grids for the $Pm\overline{3}m$, $Pbnm$, and $P6_3/mmc$ phases, respectively. The exciton parameters, including exciton binding energies, temperature, radii, and probabilities of the electron-hole wavefunction at zero separation, were calculated using the Wannier-Mott model[21]. The Fröhlich polaron model[22], and Hellwarth[23, 24] and Feynman[25, 26] theories were used to cal-

culate carrier-phonon coupling strengths, polaron radii, polaron masses, and charge carrier mobilities.

## II. STRUCTURAL STABILITY

The Goldschmidt tolerance factor $t$ is a dimensionless descriptor that is often employed to investigate the formability of perovskites[27]. We use this dimensionless descriptor to check the structural stability of the inorganic antiperovskite nitrides under investigation. $t$ is obtained by

$$t = \frac{(r_A + r_X)}{\sqrt{2}(r_B + r_X)} \tag{1}$$

where $r_A$, $r_B$, $r_X$ are the ionic radii of the anions A and B, and the cation X. Typically, $t$ is calculated using the Shannon's ionic radii. However, Shannon's ionic radii are not yet reported for anionic pnictogens $X^{3-}$ (X = N, P, As, Sb, Bi). Thus, we have used the ionic radii for $N^{3-}$, $As^{3-}$, $Sb^{3-}$ as calculated by Mochizuki *et al* [28]. The experimental lattice parameters [7–9] and their space groups are summmarized in Table I along with the computed values of $t$.

TABLE I: Space group, experimental lattice parameters, and Goldschmidt tolerance factor ($t$) of $X_3NA$ antiperovskites.

| **$X_3NA$** | **Space group** | **a (Å)** | **b (Å)** | **c (Å)** | $t$ |
|---|---|---|---|---|---|
| $Mg_3NSb$ | $Pm\overline{3}m$ | 4.35[7] | 4.35 | 4.35 | 0.94 |
| $Sr_3NSb$ | $Pm\overline{3}m$ | 5.17[9] | 5.17 | 5.17 | 0.90 |
| $Ba_3NSb$ | $P6_3/mmc$ | 7.53[9] | 7.53 | 6.64 | 0.89 |
| $Ca_3NAs$ | $Pbnm$ | 6.72[8] | 6.71 | 9.52 | 0.86 |
| $Sr_3NAs$ | $Pbnm$ | 7.15[8] | 7.18 | 10.14 | 0.85 |

## III. PHONON BAND STRUCTURES

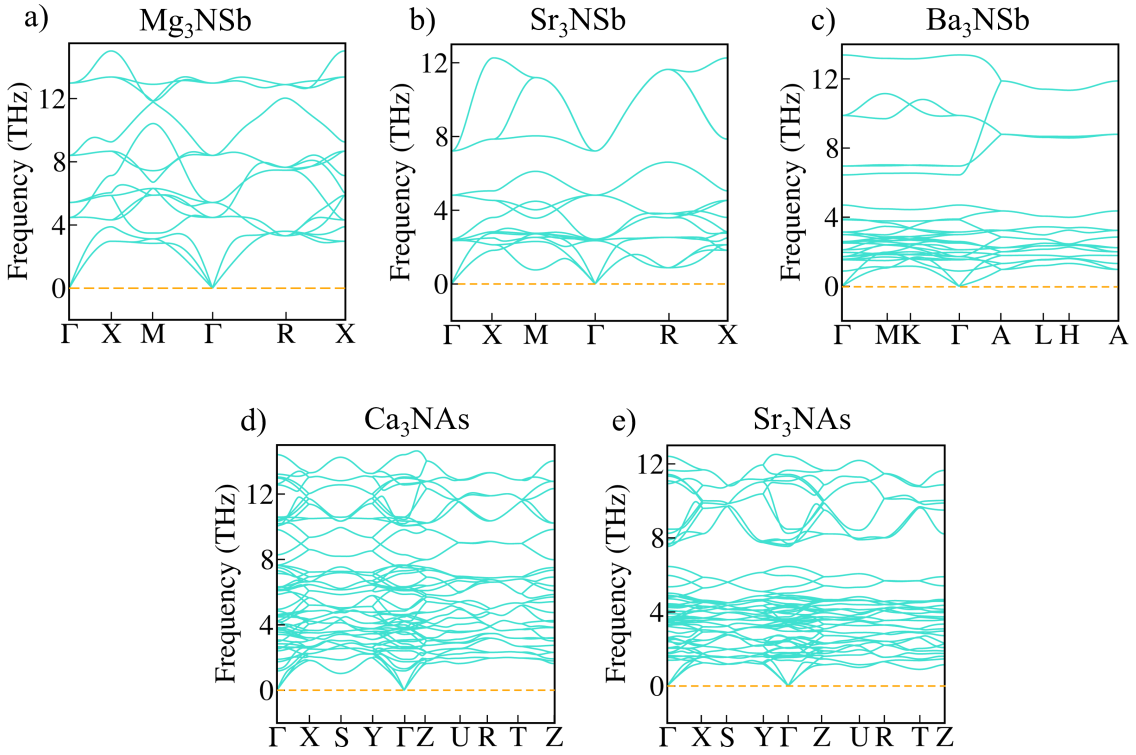


Fig.S 1: Phonon band structures obtained by DFPT for $2 \times 2 \times 2$ supercells of the $X_3NA$ antiperovskites.

## IV. ELECTRONIC BAND STRUCTURE OBTAINED BY HSE06

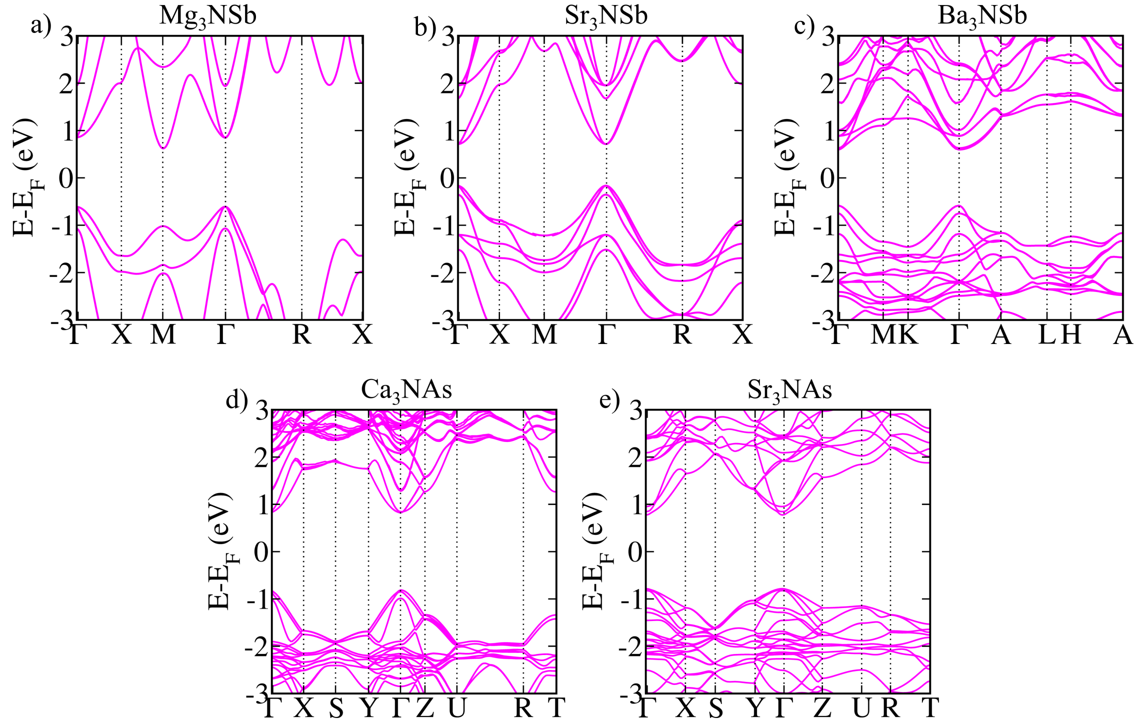


Fig.S 2: Electronic band structures of the $X_3NA$ antiperovskites obtained by HSE06.

## V. CONVERGENCE OF $G_0 W_0$ CALCULATIONS

We have performed $G_0 W_0$@PBE calculations, including spin-orbit coupling (SOC), for all investigated materials. The convergence of the band gap with the number of unoccupied bands is shown exemplarily for the case of $Mg_3NSb$ in Table II.

TABLE II: Convergence of band gap (in eV) with respect to the number of unoccupied bands (parameter NBANDS in VASP) for $Mg_3NSb$.

| **NBANDS** | $E_g$ **(eV)** |
|---|---|
| 60 | 1.04 |
| 120 | 1.14 |
| 180 | 1.15 |
| 240 | 1.14 |

## VI. CONVERGENCE OF BSE CALCULATIONS

### A. Number of orbitals

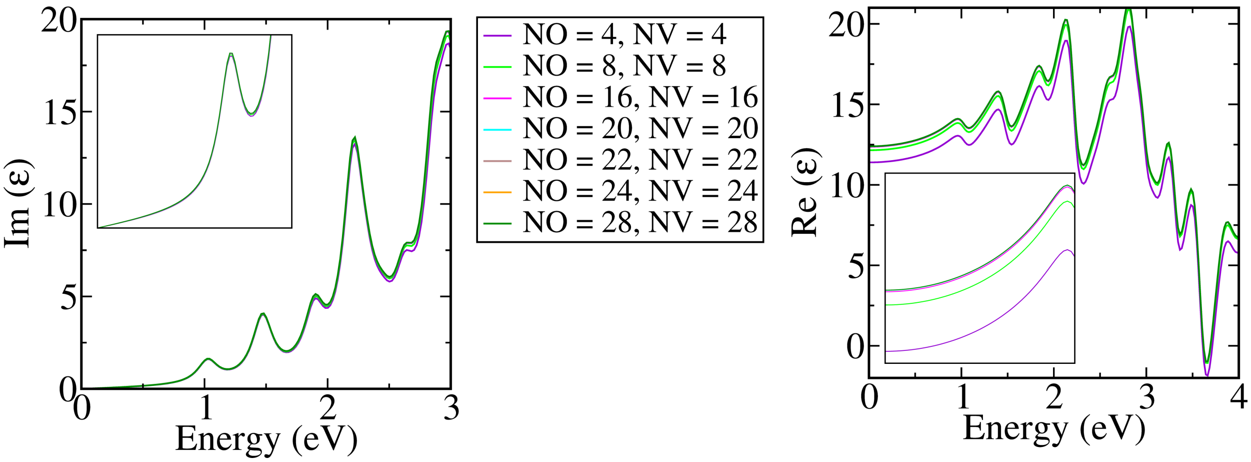


Fig.S 3: Convergence of the dielectric function of $Mg_3NSb$ with the number of occupied (NO) and unoccupied (NV) orbitals in the BSE formalism.

From Figure 3, we observe that the dielectric function converges with 16 (un)orbitals. We have used 22 in the BSE calculations for all studied antiperovskites.

## B. $k$-grid

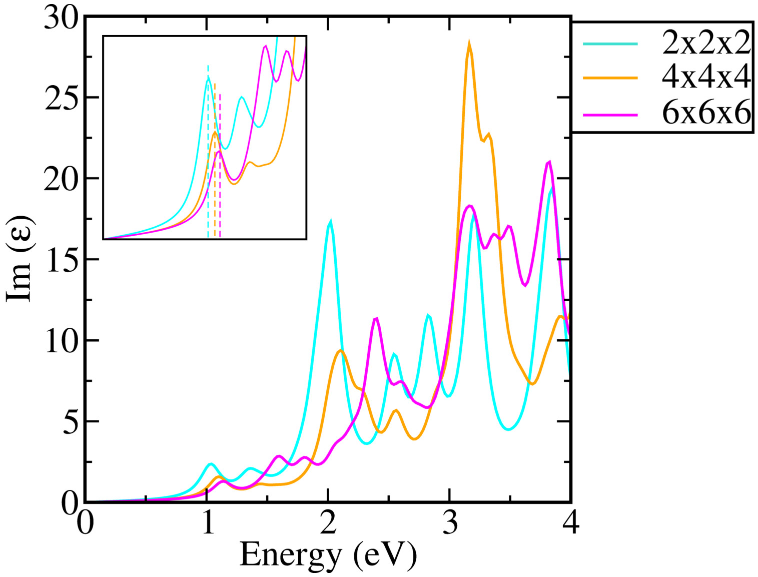


Fig.S 4: Optical spectra obtained by BSE@$G_0 W_0$@HSE06 using 2x2x2, 4x4x4, and 6x6x6 $k$-grids for $Mg_3NSb$.

The optical spectra of $Mg_3NSb$ computed with the BSE on top of $G_0 W_0$@HSE06 for 2×2×2, 4×4×4, and 6×6×6 $k$-grids are shown in Fig. 4. Due to the high computational cost required for BSE calculations, it is challenging to achieve fully converged peak positions. To present a qualitative analysis of how the $k$-grid affects the spectra and therefore the exciton binding energies, we have performed model BSE (mBSE)[29] calculations on top of PBE for $Mg_3NSb$. The mBSE approach is based on two approximations. The primary approximation is that mBSE excludes the complete RPA calculation for the momentum-dependent dielectric matrix. Additionally, it neglects the off-diagonal terms of $W_{GG'}$. Furthermore, for the construction of the BSE kernel, we apply scissor operator, which is evaluated by taking the difference between the $GW$ and the DFT band gaps. When performing mBSE calculations with increasing $k$-grid, we observe an almost 50% decrease in the value of the exciton binding energy going from the 6×6×6 to the 10×10×10 $k$-grid (see Table III). Going beyond a 10×10×10 $k$-grid was beyond our scope, especially with HSE6 as a starting point. Therefore, we have used the Wannier-Mott model[21] to calculate the exciton binding energies for the studied antiperovskites.

[h]

TABLE III: Exciton binding energy (in meV) for $Mg_3NSb$ using the mBSE approach.

| **Material** | **6×6×6** | **8×8×8** | **10×10×10** |
|---|---|---|---|
| $Mg_3NSb$ | 131.3 | 98.3 | 77.3 |

## VII. POLARON PARAMETERS

For materials with multiple scattering channels due to different longitudinal optical (LO) phonon modes, Hellwarth *et al.* [24] suggested two approximations to compute the effective LO phonon frequency $\omega_{LO,eff}$. Here, we use their athermal 'B' scheme [26] to estimate $\omega_{LO,eff}$ using the following relations:

$$\frac{W^2_{LO,eff}}{\omega^2_{LO,eff}} = \sum_{i=1}^{m} \frac{W^2_{LO,i}}{\omega^2_{LO,i}}$$

$$W^2_{LO,eff} = \sum_{i=1}^{m} W^2_{LO,i},$$

where $\omega_{LO,i}$ is the frequency of the $i^{th}$-LO mode, $W_{LO,i}$ is the weight of the $i^{th}$-LO phonon mode, and $W_{LO,eff}$ is the effective weight from all the modes.

$\omega_{LO,eff}$ is then used to evaluate the polaron mobility using Hellwarth and Feynman theories [23–26] as follows:

$$\mu = \frac{(3\sqrt{\pi}e)}{m^*\alpha\omega_{LO,eff}} \frac{\sinh\frac{\beta}{2}}{\beta^{\frac{5}{2}}} \frac{w^3}{v^3} \frac{1}{K(a,b)},$$

where, $e$ is the elementary charge, $m^*$ is the effective mass of electron or hole, $\alpha$ is the strength of electron- (or hole)-phonon coupling, and $\beta = \frac{\hbar\omega_{LO,eff}}{k_B T}$ is the reduced thermodynamic temperature in units of the phonon energy ($\hbar\omega_{LO,eff}$), with Planck's constant $\hbar$, Boltzmann constant $k_B$, and temperature $T$. $K(a,b) = \int_0^\infty du[u^2 + a^2 - bcos(vu)]^{-3/2}cos(u)$ is the polaron response to a change in the driving force, $a^2 = (\beta/2)^2 + \frac{(v^2-w^2)}{w^2 v}\beta\coth(\beta v/2)$, and $b = \frac{(v^2-w^2)}{w^2 v}\frac{\beta}{sinh(\beta v/2)}$. $w$ and $v$ are temperature-dependent variational parameters.

[1] P. Hohenberg and W. Kohn, Inhomogeneous electron gas, Phys. Rev. **136**, B864 (1964).

[2] W. Kohn and L. J. Sham, Self-consistent equations including exchange and correlation effects, Phys. Rev. **140**, A1133 (1965).

[3] G. Kresse and D. Joubert, From ultrasoft pseudopotentials to the projector augmented-wave method, Phys. Rev. B. **59**, 1758 (1999).

[4] G. Kresse and J. Furthmüller, Efficiency of ab-initio total energy calculations for metals and semiconductors using a plane-wave basis set, Comput. Mater. Sci. **6**, 15 (1996).

[5] P. E. Blöchl, Projector augmented-wave method, Phys. Rev. B. **50**, 17953 (1994).

[6] A. Gulans, S. Kontur, C. Meisenbichler, D. Nabok, P. Pavone, S. Rigamonti, S. Sagmeister, U. Werner, and C. Draxl, Exciting: a full-potential all-electron package implementing density-functional theory and many-body perturbation theory, J. Phys. Condens. Matter **26**, 363202 (2014).

[7] E. Chi, W. Kim, N. Hur, and D. Jung, New mg-based antiperovskites $PnNMg_3$ $(Pn = As, Sb)$, Solid State Commun. **121**, 309 (2002).

[8] D. Stoiber and R. Niewa, Perovskite distortion inverted: Crystal structures of $(A_3N)As$ $(A = Mg, Ca, Sr, Ba)$, Z Anorg Allg Chem. **645**, 329 (2019).

[9] F. Gäbler, M. Kirchner, W. Schnelle, U. Schwarz, M. Schmitt, H. Rosner, and R. Niewa, $(Sr_3N)E$ and $(Ba_3N)E$ $(E = Sb, Bi)$: Synthesis, crystal structures, and physical properties, Z Anorg Allg Chem. **630**, 2292 (2004).

[10] J. P. Perdew, K. Burke, and M. Ernzerhof, Generalized gradient approximation made simple, Phys. Rev. Lett. **77**, 3865 (1996).

[11] A. Togo, F. Oba, and I. Tanaka, First-principles calculations of the ferroelastic transition between rutile-type and $CaCl_2$-type $SiO_2$ at high pressures, Phys. Rev. B. **78**, 134106 (2008).

[12] A. Togo and I. Tanaka, First principles phonon calculations in materials science, Scr. Mater. **108**, 1 (2015).

[13] A. V. Krukau, O. A. Vydrov, A. F. Izmaylov, and G. E. Scuseria, Influence of the exchange screening parameter on the performance of screened hybrid functionals, J. Chem. Phys. **125**, 224106 (2006).

[14] A. M. Ganose, A. J. Jackson, and D. O. Scanlon, Sumo: Command-line tools for plotting and analysis of periodic *ab initio* calculations, J. Open Source Softw. **3**, 717 (2018).

[15] L. Hedin, New method for calculating the one-particle green's function with application to the electron-gas problem, Phys. Rev. **139**, A796 (1965).

[16] M. S. Hybertsen and S. G. Louie, First-principles theory of quasiparticles: Calculation of band gaps in semiconductors and insulators, Phys. Rev. Lett. **55**, 1418 (1985).

[17] E. E. Salpeter and H. A. Bethe, A relativistic equation for bound-state problems, Phys. Rev. **84**, 1232 (1951).

[18] M. Rohlfing and S. G. Louie, Electron-hole excitations in semiconductors and insulators, Phys. Rev. Lett. **81**, 2312 (1998).

[19] S. Albrecht, L. Reining, R. Del Sole, and G. Onida, Ab initio calculation of excitonic effects in the optical spectra of semiconductors, Phys. Rev. Lett. **80**, 4510 (1998).

[20] M. Gajdoš, K. Hummer, G. Kresse, J. Furthmüller, and F. Bechstedt, Linear optical properties in the projector-augmented wave methodology, Phys. Rev. B. **73**, 045112 (2006).

[21] G. La Rocca, Wannier–mott excitons in semiconductors, Thin Films Nanostruct. **31**, 97 (2003).

[22] H. Fröhlich, Electrons in lattice fields, Adv. Phys. **3**, 325 (1954).

[23] Y. Ōsaka, Polaron state at a finite temperature, Prog. Theor. Phys. **22**, 437 (1959).

[24] R. W. Hellwarth and I. Biaggio, Mobility of an electron in a multimode polar lattice, Phys. Rev. B. **60**, 299 (1999).

[25] R. P. Feynman, Slow electrons in a polar crystal, Phys. Rev. **97**, 660 (1955).

[26] J. M. Frost, Calculating polaron mobility in halide perovskites, Phys. Rev. B. **96**, 10.1103/physrevb.96.195202 (2017).

[27] M. R. Filip and F. Giustino, The geometric blueprint of perovskites, Proc. Natl. Acad. Sci. U.S.A. **115**, 5397 (2018).

[28] Y. Mochizuki, H.-J. Sung, A. Takahashi, Y. Kumagai, and F. Oba, Theoretical exploration of mixed-anion antiperovskite semiconductors $M_3XN$ ($M = Mg, Ca, Sr, Ba; X = P, As, Sb, Bi$), Phys. Rev. Mater. **4**, 044601 (2020).

[29] M. Bokdam, T. Sander, A. Stroppa, S. Picozzi, D. Sarma, C. Franchini, and G. Kresse, Role of polar phonons in the photo excited state of metal halide perovskites, Sci. Rep. **6**, 28618 (2016).
